# Supplementary material for: LAMD: Context-driven Android Malware Detection and Classification with LLMs
Source: arXiv:2502.13055 source file (2025-04-21)
Supplement: Supplementary file 1 [file Appendix.tex]

\section{Appendix}

% \subsection{Performance in Dataset with Different Distribution}

\subsection{Invariant Training Algorithm}
\begin{algorithm}[htb]
\caption{Algorithm of Invariant Training}
\label{alg1}
    \begin{algorithmic}[1]
    \REQUIRE ~training dataset containing $|\mathcal{E}|$ environments $\mathcal{D}_{tr}$ and each sample $x$ has a binary classification label $y_{c}, c \in [0, 1]$ and an environment label $y_e, e \in \mathcal{E}$, batch size $|\mathcal{B}|$, predefined number of epochs for stage 1 training $N$, hyperparameters $\alpha$ and $\beta$ for loss weighting, model $f$ with encoder network $\phi$ and predictor $h$. 
    \ENSURE 
    \STATE \textbf{Stage 1: Discriminative Information Amplification}
    \FOR{$\text{epoch} = 1$ to $N$}
        \FOR{$i = 1, \ldots, |\mathcal{B}|$}
            \FOR{$e \in \mathcal{E}$}
            \STATE select mini-batch of samples ${x_i^{e}} \subseteq \mathcal{B}$ \\
            \STATE calculate classification loss $\mathcal{L}^{e}_{CLS}$\\
            \STATE calculate multi-proxy contrastive loss $\mathcal{L}^{e}_{MPC}$ \\
            \ENDFOR
        \STATE obtain loss for empirical risk minimization $\mathcal{L}_{ERM} = \frac{1}{|\mathcal{E}|} \sum_{e \in \mathcal{E}} \mathcal{L}^{e}_{CLS} + \alpha \cdot \mathcal{L}^{e}_{MPC}$
        \STATE update $f$ by backpropagating $\mathcal{L}_{ERM}$
        \ENDFOR
    \ENDFOR
    \STATE \textbf{Stage 2: Unstable Information Suppression}
    \STATE Reset optimizer parameters
    \STATE Continue with model parameters from Stage 1\\
    \FOR{$\text{epoch} = N+1$ to $\text{TotalEpochs}$}
        \FOR{$i = 1, \ldots, |\mathcal{B}|$}
            \STATE get representations $\mathbf{z}_i \gets \phi(x_i)$
            \FOR{$e \in \mathcal{E}$}
            \STATE select mini-batch of representations ${\mathbf{z}_i^{e}} \subseteq \mathbf{z}_i$ \\
            \STATE initialize dummy classifier $\{s_{e} = 1.0\}$ \\
            \STATE calculate invariant gradient alignment loss $\mathcal{L}^e_{IGA}$ \\
            \ENDFOR
            \STATE get predicted labels $\tilde{y}_c \gets f(\mathbf{z}_i)$ \\
            \STATE obtain classification loss $\frac{1}{|\mathcal{E}|}\sum_{e \in \mathcal{E}}\mathcal{L}^e_{IGA}$ \\
            \STATE $\mathbf{p}_{c} \gets \text{mean}(\mathbf{z}_c),c \in [0, 1]$ \\
            \STATE obtain multi-proxy contrastive loss $\mathcal{L}_{MPC}$ \\
            \STATE $\mathcal{L}_{IRM} \gets \mathcal{L}_{CLS} + \alpha \cdot \mathcal{L}_{MPC} + \beta \cdot \frac{1}{|\mathcal{E}|}\sum_{e \in \mathcal{E}}\mathcal{L}^e_{IGA}$ \\
            \STATE update $f$ by backpropagating $\mathcal{L}_{IRM}$
        \ENDFOR
    \ENDFOR
    \end{algorithmic}
\end{algorithm}

The proposed invariant training process is shown in Algorithm~\ref{alg1}. This learning framework consists of two phases: discriminative information amplification and unstable information suppression. In Stage 1, the model enhances its ability to learn discriminative features through empirical risk minimization (ERM). Specifically, in Line 6, the classification loss $\mathcal{L}^{e}_{CLS}$ is calculated for each environment to ensure correct class separation, and in Line 7, a multi-proxy contrastive loss $\mathcal{L}^{e}_{MPC}$ is computed to improve the discriminative power among samples. The combined loss for ERM, including the classification and contrastive components, is computed in Line 10, and then the model is updated by backpropagation in Line 11. Stage 2 focuses on suppressing unstable information through invariant training. In Line 13, the optimizer is reset to remove the influence of previous training, while the model parameters from Stage 1 are retained in Line 14 to preserve the learned discriminative capabilities. Line 17 extracts sample representations through the encoder, and Line 21 calculates the invariant gradient alignment (IGA) loss $\mathcal{L}^e_{IGA}$ for each environment, which ensures similar responses across environments. The combined invariant risk minimization (IRM) loss is formed in Line 28, integrating the classification, contrastive, and alignment losses, followed by updating the model in Line 29. This two-phase training process enables the model to learn features that are both discriminative and stable, improving robustness and generalization in the face of distribution drift.
